# Supplementary material for: Neural Network Learner for Minesweeper
Source: arXiv:2212.10446 source file (2022-11-30)
Supplement: Supplementary file 1 [file appendix_A.tex]

\chapter{An Appendix Chapter (Optional)}
\label{appn:A}
% Optional chapter
Some lengthy tables, codes, raw data, length proofs, etc. which are \textbf{very important but not essential part} of the project report goes into an Appendix. An appendix is something a reader would consult if he/she needs extra information and a more comprehensive understating of the report. Also, note that you should use one appendix for one idea.

An appendix is optional. If you feel you do not need to include an appendix in your report, avoid including it. Sometime including irrelevant and unnecessary materials in the Appendices may unreasonably increase the total number of pages in your report and distract the reader.
