# Supplementary material for: Neural Network Learner for Minesweeper
Source: arXiv:2212.10446 source file (2022-11-30)
Supplement: Supplementary file 2 [file appendix_B.tex]

\chapter{An Appendix Chapter (Optional)}
\label{appn:B}

...
